# Supplementary material for: Constructing the general partial waves and renormalization in EFT
Source: arXiv:2111.08019 ancillary file (2022-10-10)
Supplement: Supplementary file 1 [file supplement.pdf]

## GENERAL PARTIAL-WAVE BASIS AND PARTIAL-WAVE EXPANSION

In this section, we first construct the CG coefficients and partial-wave amplitude basis with $J < 2$ of scattering $\psi_1^\dagger\psi_2^\dagger \to \phi_3\phi_4\phi_5$ and $\psi_1^\dagger\phi_2\phi_3 \to \psi_4^\dagger\phi_5$. By the equations in the main text, we list the formula in Tab. 1

| $\psi_1^\dagger\psi_2^\dagger\phi_3 \to \phi_4\phi_5$ | | | |
|---|---|---|---|
| $J_{45}$ | CG coefficients | | partial-wave basis |
| 0 | $\mathcal{C}_{\rm L} = [12]$ | $\mathcal{C}_{\rm R} = 1$ | $\mathcal{B}^0 = [12]$ |
| 1 | $\mathcal{C}_{\rm L1}^{\{I_1,I_2\}} = \frac{1}{\sqrt{2s_{45}}}[1\boldsymbol{x}^{\{I_1}][2\boldsymbol{x}^{I_2\}}]$<br>$\mathcal{C}_{\rm L2}^{\{I_1,I_2\}} = \frac{1}{\sqrt{2s_{45}}}[12][3\boldsymbol{x}^{\{I_1}]\langle 3\boldsymbol{x}^{I_2\}}\rangle$<br>$\mathcal{C}_{\rm L3}^{\{I_1,I_2\}} = \frac{1}{\sqrt{2s_{45}}}[13][2\boldsymbol{x}^{\{I_1}]\langle 3\boldsymbol{x}^{I_2\}}\rangle$ | $\mathcal{C}_{{\rm R},\{I_1,I_2\}} = \frac{1}{\sqrt{2}s_{45}^{3/2}}[\boldsymbol{x}_{\{I_1}4][\boldsymbol{x}_{I_2\}}5]\langle 45\rangle$ | $\mathcal{B}_1^1 = \frac{1}{s_{45}}\langle 45\rangle\,([14][25]+[15][24])$<br>$\mathcal{B}_2^1 = \frac{1}{s_{45}}[12](s_{34}-s_{35})$<br>$\mathcal{B}_3^1 = \frac{1}{s_{45}}[13]([24]\langle 34\rangle - [25]\langle 35\rangle)$ |

| $\psi_1^\dagger\phi_2\phi_3 \to \psi_4^\dagger\phi_5$ | | | |
|---|---|---|---|
| $J_{45}$ | CG coefficients | | partial-wave basis |
| 1/2 | $\mathcal{C}_{\rm L1}^{1/2} = [1\boldsymbol{x}]$<br>$\mathcal{C}_{\rm L2}^{1/2} = \frac{1}{s_{45}}[12]\langle 23\rangle[3\boldsymbol{x}]$ | $\mathcal{C}_{\rm R}^{1/2} = [\boldsymbol{x}4]/\sqrt{s_{45}}$ | $\mathcal{B}_1^{1/2} = [14]$<br>$\mathcal{B}_2^{1/2} = \frac{1}{s_{45}}[12]\langle 23\rangle[34]$ |
| 3/2 | $\mathcal{C}_{\rm L1}^{3/2} = \frac{1}{\sqrt{3}s_{45}^{3/2}}\langle 12\rangle[1\boldsymbol{x}][1\boldsymbol{x}][2\boldsymbol{x}]$<br>$\mathcal{C}_{\rm L2}^{3/2} = \frac{1}{\sqrt{3}s_{45}^{3/2}}\langle 13\rangle[1\boldsymbol{x}][1\boldsymbol{x}][3\boldsymbol{x}]$<br>$\mathcal{C}_{\rm L3}^{3/2} = \frac{1}{\sqrt{6}s_{45}^{3/2}}\langle 23\rangle[1\boldsymbol{x}][2\boldsymbol{x}][3\boldsymbol{x}]$<br>$\mathcal{C}_{\rm L4}^{3/2} = \frac{1}{\sqrt{3}s_{45}^{5/2}}\langle 23\rangle^2[12][2\boldsymbol{x}][3\boldsymbol{x}][3\boldsymbol{x}]$ | $\mathcal{C}_{\rm R}^{3/2} = \frac{1}{\sqrt{3}s_{45}^2}[\boldsymbol{x}4][\boldsymbol{x}4][\boldsymbol{x}5]\langle 45\rangle$ | $\mathcal{B}_1^{3/2} = \frac{1}{s_{45}^2}\langle 12\rangle\langle 45\rangle\left([14]^2[25]+2[14][15][24]\right)$<br>$\mathcal{B}_2^{3/2} = \frac{1}{s_{45}^2}\langle 13\rangle\langle 45\rangle\left([14]^2[35]+2[14][15][34]\right)$<br>$\mathcal{B}_3^{3/2} = \frac{\sqrt{2}}{s_{45}^2}\langle 23\rangle\langle 45\rangle\left([14][24][35]+[14][25][34]+[15][24][34]\right)$<br>$\mathcal{B}_4^{3/2} = \frac{1}{s_{45}^3}\langle 23\rangle^2\langle 45\rangle[12]\left([25][34]^2+2[24][34][35]\right)$ |

TABLE I. The $J < 2$ CG coefficients and partial-wave amplitude basis of scattering $\psi_1^\dagger\psi_2^\dagger \to \phi_3\phi_4\phi_5$ and $\psi_1^\dagger\phi_2\phi_3 \to \psi_4^\dagger\phi_5$

The same is true for higher-$J$ basis. Then the partial-wave expansion of any amplitude in this type is below.

$$\mathcal{A}(\psi_1^\dagger,\psi_2^\dagger,\phi_3 \to \phi_4,\phi_5) = \mathcal{M}_0\left(s_{12},s_{13},s_{23}\right)\mathcal{B}^{J=0} + \mathcal{M}_{11}\mathcal{B}_1^{J=1} + \mathcal{M}_{12}\mathcal{B}_2^{J=1} + \mathcal{M}_{13}\mathcal{B}_3^{J=1} + \sum_{J>1}\mathcal{M}_{Ji}\mathcal{B}_i^J . \quad (1)$$

The coefficients $\mathcal{M}_{Ji}$ are the function of $\{s_{12},s_{13},s_{23}\}$, which are independent and do not affact the angular momentum $J$ in this channel.

Then we focus on the partial-wave expansion for $\psi_1^\dagger\phi_2\phi_3 \to \psi_4^\dagger\phi_5$ to demonstrate the expansion for factorizable amplitudes. The solution can be applied directly to the integral in the next section.

We reduce $\mathcal{A}_D = \frac{1}{\langle 14\rangle}$ as the first example with the formula

$$\int d\Phi_{1',2'} \oint_\infty \frac{dz}{z}\,\hat{\mathcal{C}}^J(z)\hat{\mathcal{A}}(z) = g_2(J)\sum_a \mathcal{M}_{\rm reg}^{J,a}\mathcal{C}_{\bar{f}}^{J,a} . \quad (2)$$

$$\frac{4}{\pi}\int d\Phi_{4,5}\ \mathcal{A}_D\cdot\left(\mathcal{C}^{1/2}_{\rm R}\right)^* = \frac{-2}{s_{12}+s_{13}}[1\boldsymbol{x}] = \frac{2}{s_{12}+s_{13}}\mathcal{C}^{1/2}_{\rm L}, \tag{3}$$

$$\begin{aligned}\frac{8}{\pi}\int d\Phi_{4,5}\ \mathcal{A}_D\cdot\left(\mathcal{C}^{3/2}_{\rm R}\right)^* &= \frac{8}{\pi s_{45}^2}\frac{\pi}{4}\frac{\langle 45\rangle[45]\langle 1\boldsymbol{x}\rangle\left([1|p_{\boldsymbol{x}}|\boldsymbol{x}\rangle\right)^2}{\sqrt{3}(s_{12}+s_{13})^2}\\ &= \frac{2}{\sqrt{3}\sqrt{s_{45}}(s_{12}+s_{13})^2}\left(\langle 12\rangle[2\boldsymbol{x}][1\boldsymbol{x}][1\boldsymbol{x}]+\langle 13\rangle[3\boldsymbol{x}][1\boldsymbol{x}][1\boldsymbol{x}]\right)\\ &= \frac{2s_{45}}{(s_{12}+s_{13})^2}\left(\mathcal{C}^{3/2}_{\rm L1}+\mathcal{C}^{3/2}_{\rm L2}\right).\end{aligned} \tag{4}$$

Herein

$$\mathcal{A}_D = \frac{-2}{s_{12}+s_{13}}\mathcal{B}^{1/2}+\frac{2s_{45}}{(s_{12}+s_{13})^2}\mathcal{B}^{3/2}_1+\frac{2s_{45}}{(s_{12}+s_{13})^2}\mathcal{B}^{3/2}_2 + \sum_{J\geq 5/2}\mathcal{M}_{Ji}\mathcal{B}^J_i. \tag{5}$$

Which is applied to eq. (??). But not all factorizable amplitudes have to be reduced by integral. Using eq. (5), production of arbitrary local amplitude $\mathcal{A}_N$ and $\mathcal{A}_D$ can be expanded algebraically. Note that $\mathcal{A}_N\mathcal{B}^J$ can only contain partial waves in the range $\left[|J-J_N|, J+J_N\right]$ due to the angular momentum algebra, it is safe the truncate the expansion of $\mathcal{A}_N\mathcal{A}_D$ when we are only interested in the low $J$'s. For instance, based on the result eq. (5), take $\mathcal{A}_N=[2|p_3-p_5|4\rangle$ with $J_N=1/2$. The expansion is given as

$$\begin{aligned}\frac{\mathcal{A}_N}{\langle 14\rangle} =& \frac{-2}{s_{12}+s_{13}}\mathcal{A}_N\mathcal{B}^{1/2}+\frac{2s_{45}}{(s_{12}+s_{13})^2}\mathcal{A}_N(\mathcal{B}^{3/2}_1+\mathcal{B}^{3/2}_2)+\sum_{J\geq 5/2}\mathcal{M}_{Ji}\mathcal{A}_N\mathcal{B}^J_i\\ =& \frac{-2}{s_{12}+s_{13}}\left(\left(-\frac{1}{2}s_{12}-\frac{1}{2}s_{13}-s_{23}\right)\mathcal{B}_0+\frac{1}{2}s_{45}\left(\mathcal{B}^1_1+\mathcal{B}^1_2+\mathcal{B}^1_3\right)\right)\\ &+\frac{2s_{45}}{(s_{12}+s_{13})^2}\left(\frac{1}{2}\left(s_{12}+s_{13}+3s_{23}\right)\mathcal{B}^1_1-\left(s_{12}+s_{13}+\frac{3}{2}s_{23}\right)\left(\mathcal{B}^1_2+\mathcal{B}^1_3\right)\right)\\ &+\sum_{J\geq 5/2}\mathcal{M}_{Ji}\mathcal{A}_N\mathcal{B}^J_i\\ =& \left(1+\frac{2s_{23}}{s_{12}+s_{13}}\right)\mathcal{B}^0+\frac{3s_{45}s_{23}}{(s_{12}+s_{13})^2}\mathcal{B}^1_1-\frac{3s_{45}^2}{(s_{12}+s_{13})^2}\mathcal{B}^1_2-\frac{3s_{45}^2}{(s_{12}+s_{13})^2}\mathcal{B}^1_3+\sum_{J\geq 2}\mathcal{M}'_{Ji}\mathcal{B}^J_i.\end{aligned} \tag{6}$$

Where $\mathcal{B}^0$ and $\mathcal{B}^1_i$ are the same as in Tab. 1.

## SMEFT TREE AMPLITUDES

In this section, we present all the tree-level amplitudes in the SMEFT that will be used as subamplitudes of unitarity cuts. Derive from $\mathcal{L}$.

$$\begin{aligned}\mathcal{L} =& (\text{kinetic terms}) - Y_e(\bar{e}lH^\dagger) - Y_e^\dagger(\bar{l}eH) - \lambda(H^\dagger H)^2\\ &+ C_{He}(\bar{e}\gamma^\mu e)(H^\dagger i\overleftrightarrow{D}_\mu H) + C_{eH}(\bar{l}eH)(H^\dagger H) + \dots\end{aligned} \tag{7}$$

Where the tree amplitudes generated by the pure SM are

$$\mathcal{A}_{sm}(H^{\dagger i}, H_j, H^{\dagger k}, H_l) = -2\lambda\left(\delta^i_j\delta^k_l+\delta^i_l\delta^k_j\right), \tag{8}$$

$$\begin{aligned}\mathcal{A}_{sm}(\bar{l}^i_p, e_r, H_j, H^{\dagger k}, H_l) =& -2[Y_e^\dagger]_{pr}\lambda\left(\delta^i_j\delta^k_l+\delta^i_l\delta^k_j\right)\frac{1}{\langle 12\rangle}\\ &+[Y_e^\dagger Y_e Y_e^\dagger]_{pr}\delta^i_l\delta^k_j\frac{\langle 35\rangle}{\langle 15\rangle\langle 23\rangle}-[Y_e^\dagger Y_e Y_e^\dagger]_{pr}\delta^i_j\delta^k_l\frac{\langle 35\rangle}{\langle 13\rangle\langle 25\rangle},\end{aligned} \tag{9}$$

$$\mathcal{A}_{sm}(\bar{l}^i_p, H^{\dagger k}, l_{r,j}, H_l) = -[Y_e^\dagger Y_e]_{pr}\delta^i_l\delta^k_j\frac{[12]}{[23]}, \tag{10}$$

$$\mathcal{A}_{sm}(H^{\dagger i}, H_j, \bar{e}_p, e_r) = -[Y_e Y_e^\dagger]_{pr}\delta^i_j\frac{[14]}{[13]}. \tag{11}$$

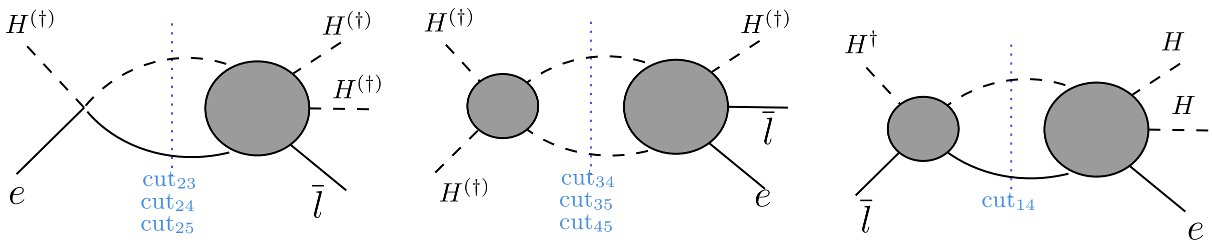


FIG. 1. All the double cuts of the one-loop amplitude that contributes to $\dot{C}_{eH}$. The gray blobs are tree-level on-shell amplitudes.

The amplitudes involved by the effective operators are expressed as

$$\mathcal{A}_{eH}(\bar{l}^i, e, H_j, H^{\dagger k}, H_l) = C_{eH}\left(\delta^i_j\delta^k_l + \delta^i_l\delta^k_j\right)[12]. \quad (12)$$

$$\mathcal{A}_{He}(\bar{e}, e, H^{\dagger i}, H_j) = C_{He}\delta^i_j[2|p_4 - p_3|1\rangle, \quad (13)$$

$$\mathcal{A}_{He}(\bar{l}^i_p, e_r, H_j, H^{\dagger k}, H_l) = [Y_e^\dagger C_{He}]_{pr}\delta^i_j\delta^k_l\frac{\langle 3|p_5 - p_4|2]}{\langle 13\rangle} + [Y_e^\dagger C_{He}]_{pr}\delta^i_l\delta^k_j\frac{\langle 5|p_3 - p_4|2]}{\langle 15\rangle}, \quad (14)$$

$$\mathcal{A}_{He}(\bar{l}^i_p, H_j, e_r, \bar{e}_s, e_t) = -[Y_e^\dagger]_{pt}[C_{He}]_{sr}\delta^i_j\frac{2\langle 4|2|3]}{\langle 15\rangle} + [Y_e^\dagger]_{pr}[C_{He}]_{st}\delta^i_j\frac{2\langle 4|2|5]}{\langle 13\rangle}\ . \quad (15)$$

## REG INTEGRATION

The remains are pretty straightforward by partial-wave expansion. We pick up the correct compoment of the sub-amplitudes in Fig. 1, and put them together in Tab. II. Most of them are exactly the same as eq. (5,6). Notice that the partial-wave basis in cut$_{34}$ and cut$_{45}$ with the intermediate states $e, \bar{e}$ are obtained after doing the BCFW shift.

$$\text{cut}_{45}\mathcal{A} = [Y_e^\dagger Y_e Y_e^\dagger C_{He}]\delta^j_i\delta^l_k\int d\Phi_{1',2'}\oint_{\text{Inf}}\frac{dz}{z}\frac{[42']}{[4\hat{1}'_z]}\cdot\frac{2\langle\hat{2}'_z|3|2]}{\langle 11'\rangle} \quad (16)$$

The BCFW deformation here is chosen as $|\hat{2}'_z\rangle = |2'\rangle + z|1'\rangle$, $|\hat{1}'_z] = |1'] - z|2']$. The the residue in $z\to\infty$ is $\frac{2\langle 1'|3|2]}{\langle 1'1\rangle}$, which can be decomposed by eq. (6)

Finally, We sum up the CG coefficientsin Tab. II.

$$\begin{aligned}\frac{dC_{eH}}{d\log\mu} &= -\frac{1}{8\pi^2}\sum_{\mathcal{I}}\frac{1}{2J_{\mathcal{I}}+1}\mathcal{M}_{\rm L}^{J_{\mathcal{I}}}\mathcal{M}_{\rm R}^{J_{\mathcal{I}}}\\ &= -\frac{1}{8\pi^2}\times\frac{1}{2}\Big((2[Y_e^\dagger C_{He}]\lambda)\frac{4s_{23}}{s_{14}+s_{15}}\\ &\quad - 2[Y_e^\dagger C_{He}]\lambda\frac{4s_{24}}{s_{13}+s_{15}} + \cdots\Big)\\ &\quad -\frac{1}{8\pi^2}\Big(2\lambda[Y_e^\dagger C_{He}]\left(1+\frac{2s_{25}}{s_{12}+s_{15}}\right)+\cdots\Big)\\ &= -\frac{\lambda}{4\pi^2}[Y_e^\dagger C_{He}] - \frac{1}{8\pi^2}[Y_e^\dagger Y_e Y_e^\dagger C_{He}].\end{aligned} \quad (17)$$

| $\mathcal{I}$ | state $\{1', 2'\}$ | $J$ | partial-wave basis $\mathcal{B}$ | coefficients $\mathcal{M}$ |
|---|---|---|---|---|
| (23) | $\{e, H\}$ | 1/2 | $\mathcal{B}_{\mathrm{L}} = -s_{23}^{-1}\delta^{j}_{j'}[2\|3\|1'\rangle$ | $\mathcal{M}_{\mathrm{L}} = 2C_{He}s_{23}$ |
| | | | $\mathcal{B}_{\mathrm{R}} = [1'1]\left(\delta^{j'}_{i}\delta^{l}_{k} + \delta^{l}_{i}\delta^{j'}_{k}\right)$ | $\mathcal{M}_{\mathrm{R}} = (2Y_e^\dagger\lambda + \frac{1}{2}[Y_e^\dagger Y_e Y_e^\dagger])\frac{2}{s_{14}+s_{15}}$ |
| (24) | $\{e, H\}$ | 1/2 | $\mathcal{B}_{\mathrm{L}} = -s_{24}^{-1}[2\|4\|1'\rangle\delta^{k'}_{k}$ | $\mathcal{M}_{\mathrm{L}} = -2C_{He}s_{24}$ |
| | | | $\mathcal{B}_{\mathrm{R}} = [1'1]\left(\delta^{j}_{i}\delta^{l}_{k'} + \delta^{l}_{i}\delta^{j}_{k'}\right)$ | $\mathcal{M}_{\mathrm{R}} = 2Y_e^\dagger\lambda\frac{2}{s_{13}+s_{15}}$ |
| (25) | $\{e, H\}$ | 1/2 | $\mathcal{B}_{\mathrm{L}} = -s_{25}^{-1}[2\|5\|1'\rangle\delta^{l}_{l'}$ | $\mathcal{M}_{\mathrm{L}} = 2C_{He}s_{25}$ |
| | | | $\mathcal{B}_{\mathrm{R}} = [1'1]\left(\delta^{j}_{i}\delta^{l'}_{k} + \delta^{l'}_{i}\delta^{j'}_{k}\right)$ | $\mathcal{M}_{\mathrm{R}} = (2Y_e^\dagger\lambda + \frac{1}{2}[Y_e^\dagger Y_e Y_e^\dagger])\frac{2}{s_{13}+s_{14}}$ |
| (14) | $\{e, H\}$ | 1/2 | $\mathcal{B}_{\mathrm{L}} = s_{14}^{-1}[1\|4\|1'\rangle\delta^{i'}_{i}\delta^{k'}_{k}$ | $\mathcal{M}_{\mathrm{L}} = -2[Y_e^\dagger Y_e]$ |
| | | | $\mathcal{B}_{\mathrm{R}} = [1'2]\left(\delta^{j}_{i'}\delta^{l}_{k'} + \delta^{l}_{i'}\delta^{j}_{k'}\right)$ | $\mathcal{M}_{\mathrm{R}} = -C_{He}Y_e^\dagger$ |
| (34) | $\{H^\dagger, H\}$ | 0 | $\mathcal{B}_{\mathrm{L}} = \delta^{j}_{k}\delta^{k'}_{j'} + \delta^{k'}_{k}\delta^{j}_{j'}$ | $\mathcal{M}_{\mathrm{L}} = -2\lambda$ |
| | | | $\mathcal{B}_{\mathrm{R}} = [12]\delta^{j'}_{i}\delta^{l}_{k'}$ | $\mathcal{M}_{\mathrm{R}} = -[Y_e^\dagger C_{He}]\left(1 + \frac{2s_{25}}{s_{12}+s_{15}}\right)$ |
| | $\{\bar{e}, e\}$ | 0 | $\mathcal{B}_{\mathrm{L}} = \delta^{j}_{k}\delta^{k'}_{j'} + \delta^{k'}_{k}\delta^{j}_{j'}$ | $\mathcal{M}_{\mathrm{L}} = [Y_e^\dagger Y_e]$ |
| | | | $\mathcal{B}_{\mathrm{R}} = [12]\delta^{j'}_{i}\delta^{l}_{k'}$ | $\mathcal{M}_{\mathrm{R}} = [Y_e^\dagger C_{He}]\frac{s_{25}}{s_{12}+s_{15}}$ |
| (35) | $\{H^\dagger, H\}$ | 0 | $\mathcal{B}_{\mathrm{L}} = \delta^{j}_{j'}\delta^{l}_{l'} + \delta^{j}_{l'}\delta^{l}_{j'}$ | $\mathcal{M}_{\mathrm{L}} = -2\lambda$ |
| | | | $\mathcal{B}_{\mathrm{R}} = [12]\delta^{j'}_{i}\delta^{l'}_{k}$ | $\mathcal{M}_{\mathrm{R}} = [Y_e^\dagger C_{He}]\left(1 + \frac{2s_{24}}{s_{12}+s_{14}}\right)$ |
| (45) | $\{H^\dagger, H\}$ | 0 | $\mathcal{B}_{\mathrm{L}} = \delta^{l}_{k}\delta^{k'}_{l'} + \delta^{k'}_{k}\delta^{l}_{l'}$ | $\mathcal{M}_{\mathrm{L}} = -2\lambda$ |
| | | | $\mathcal{B}_{\mathrm{R}} = [12]\delta^{l'}_{i}\delta^{j}_{k'}$ | $\mathcal{M}_{\mathrm{R}} = -[Y_e^\dagger C_{He}]\left(1 + \frac{2s_{23}}{s_{12}+s_{13}}\right)$ |
| | $\{\bar{e}, e\}$ | 0 | $\mathcal{B}_{\mathrm{L}} = \delta^{l}_{k}\delta^{k'}_{l'} + \delta^{k'}_{k}\delta^{l}_{l'}$ | $\mathcal{M}_{\mathrm{L}} = [Y_e^\dagger Y_e]$ |
| | | | $\mathcal{B}_{\mathrm{R}} = [12]\delta^{l'}_{i}\delta^{j}_{k'}$ | $\mathcal{M}_{\mathrm{R}} = [Y_e^\dagger C_{He}]\frac{s_{23}}{s_{12}+s_{13}}$ |

TABLE II. Partial wave expansions relevant for the computation of $\gamma_{He,eH}$. The first three columns list the cut channels, intermediate states and the angular momenta that are summed over in eq. (**??**). In each case, we present the partial wave bases $\mathcal{B}_{\mathrm{L/R}}$ and the coefficients $\mathcal{M}_{\mathrm{L/R}}$ of the left/right subamplitudes. Note that $C_{He}$, $Y_e$ and $Y_e^\dagger$ are the flavor tensors. The square brackets around them denote a matrix multiplication.
